# Supplementary material for: SciNews: From Scholarly Complexities to Public Narratives -- A Dataset for Scientific News Report Generation
Source: arXiv:2403.17768 source file (2024-12-10)
Supplement: Supplementary file 1 [file appendix.tex]

% \chapter{Appendix}
\section*{Human Evaluation Guideline}

Here, we offer a more detailed explanation of each metric and evaluation criterion used in our human assessment.

\textbf{Prerequisites:} If you do not satisfy both of the following requirements simultaneously: (1) at least a master's or Ph.D. student in Computer Science or Computational Linguistics, and (2) demonstrating proficiency in English, then you do not meet the qualifications for this human evaluation, and we kindly ask you not to proceed with this task. If you do meet both of the aforementioned criteria, please proceed and read the subsequent instructions.

We invite you to carefully review the following scientific paper along with four candidate news articles. Among these articles, one has been crafted by a human writer, while the remaining three have been produced by automated scientific news narrative generation models. Please note that the arrangement of these candidates is randomized for an unbiased evaluation. Once you have thoroughly read each candidate article, we request you to rate each of the following four criteria from 1 to 3, with higher ratings indicating better quality.

\begin{itemize}
    \item \textbf{Relevance:} This metric indicates whether the candidate content reflects the content of the source text well. Generated news article should contain topics relevant to the source text. For instance, if the source text discusses the impact of climate change on polar bear habitat, the relevant news article should discuss the climate change/polar bear habitat, but not other topics. Relevance is more of a macro-level evaluation, assessing how well the various topics in the candidate align with those in the original article and to what extent. Please rate the candidate in terms of relevance according to the following instructions:
    
    \begin{enumerate}
        \item Only a small fraction of the content provided by the candidate is relevant to the topic.
        \item Some content provided by the candidate is relevant to the topic, while some is not.
        \item Nearly all of the content provided by the candidate is relevant to the topic.
    \end{enumerate}
    
    \item \textbf{Simplicity:} This metric indicates the extent to which the candidate is understandable and accessible to lay readers. Candidates should convey information in a manner that is accessible to readers devoid of specialized domain knowledge. Consequently, the explanation of concepts and terms should make it easier for people to understand. For example, if the source text discusses ``photosynthesis," a simplified sentence might explain it as ``a process used by plants to convert sunlight into energy, essential for their growth and survival." Conversely, utilizing technical jargon, such as ``Photons engage in a series of photo-physical and photo-chemical events culminating in the conversion of carbon dioxide into glucose," without further explanation or example, may alienate readers who are not familiar with biological terminology, thus failing to meet the criterion of presenting information in a layman's tune. Please rate the candidate in terms of simplicity according to the following instructions:

    \begin{enumerate}
        \item The candidate is hard to understand without domain knowledge.
        \item The candidate is overall readable, with some concepts and terms not explained.
        \item The candidate is fully understandable to the layperson, all information is translated to a layman's tune.
    \end{enumerate}
    
    \item \textbf{Conciseness:} This metric indicates the extent to which the candidate omits less important information from the source text. Candidates who excel in meeting this criterion should exclude non-essential content derived from the source document during the generation process. An attempt to include all details indiscriminately should incur a reduction in the assigned score. For example, if the source document talks a lot about the technical specifications of a new gadget, a high-scoring news article might focus on highlighting the groundbreaking features and how they benefit users while omitting minutiae such as the specific materials used in internal components. Conversely, a generated news article that tries to include every single piece of information from the source, without considering the main topic or message, would not align with the criteria of a high-scoring output, hence meriting a deduction in points. Please rate the candidate in terms of conciseness according to the following instructions:
    
    \begin{enumerate}
        \item  Much of the content provided by the candidate is redundant or unimportant.
        \item Only a few points of the content provided by the candidate are redundant.
        \item Almost none of the content provided by the candidate is redundant.
    \end{enumerate}

    \item \textbf{Faithfulness:} This metric indicates the extent to which the candidate is incorrect in that it contradicts the information from the source text. Candidate should stick to the information provided in the source document and avoid adding general knowledge. If the news article includes facts that are not confirmed or contradicted by the document, it shows a lack of accuracy and will get a lower score.  For example, if the source text talks about the economic effects of a new policy but does not mention the historical context, a high-quality news article should only discuss the economic analysis mentioned in the document and not include well-known historical events related to the policy. In contrast, a news article that includes commonly known information on the historical events leading up to the policy, which is not discussed or contradicted in the source document, would display a lower level of faithfulness to the original text, thereby meriting a decrement in its evaluation score. Faithfulness involves a finer evaluation, focusing on whether the sentences in the candidate contain unsupported or contradictory content in relation to the original text. Please rate the candidate in terms of faithfulness according to the following instructions:
    
    \begin{enumerate}
        \item Much of the content provided by the candidate includes hallucinations and factual errors.
        \item Some content provided by the candidate can be supported by the source document, while some cannot.
        \item Nearly all of the content provided by the candidate is faithful/supported by the source document.
    \end{enumerate}
\end{itemize}

After that, you are also supposed to choose the best and the worst candidates according to their overall quality and predict which one is written by human.
